# Supplementary material for: O1-Pruner: Length-Harmonizing Fine-Tuning for O1-Like Reasoning Pruning
Source: arXiv:2501.12570 source file (2025-01-29)
Supplement: Supplementary file 1 [file supplementary.tex]

\onecolumn
\rule{\textwidth}{0.4pt}
{\centering\LARGE\bfseries Supplementary Material for ``O1-Pruner: Length-Harmonizing Fine-Tuning for O1-Like Reasoning Pruning" \par}
\rule{\textwidth}{0.4pt}

\section{Training Details}
For both models, we selected 5,000 problems from the MATH trainset as training data. For each problem, multiple samples were taken to generate different solutions. For each problem, Marco-o1 model samples for 16 times, while the QwQ model samples for 12 times. From each set of solutions, we randomly selected 2 solutions for training. After computing the rewards, we normalized the reward values. Marco-o1 is trained with 4 * A800-80G GPUs and QwQ-32B is trained with 8 * A800-80G GPUs. The other hyperparameters used in the training process are presented in the table below.
\begin{table}[ht]
\centering
\caption{Hyperparameters for the Marco-o1-7B and QwQ-32B-Preview models.}
\label{tab:hyperparameters}
\begin{tabular}{lcc}
\hline
\textbf{Hyperparameter}   & \textbf{Marco-o1-7B} & \textbf{QwQ-32B-Preview} \\ \hline
clip\_range               & 0.2                  & 0.2                       \\ 
$\lambda$                 & 2                    & 5                         \\ 
cutoff\_len               & 3072                 & 4096                      \\ 
batch\_size               & 32                   & 32                        \\ 
learning\_rate            & 2.0e-7               & 1.0e-6                    \\ 
num\_train\_epochs        & 1.0                  & 1.0                       \\ 
lr\_scheduler\_type       & cosine               & cosine                    \\ 
warmup\_ratio             & 0.1                  & 0.1                       \\ \hline
\end{tabular}
\end{table}

\section{Case Study}
We also present a case study of generated samples, for which we have chosen two problems each from the two models utilized in the training. These samples encompass outputs from both the base model and the model refined by the O1-Pruner optimization.
\begin{figure*}[htbp]
\centering
\includegraphics[width=5.5in]{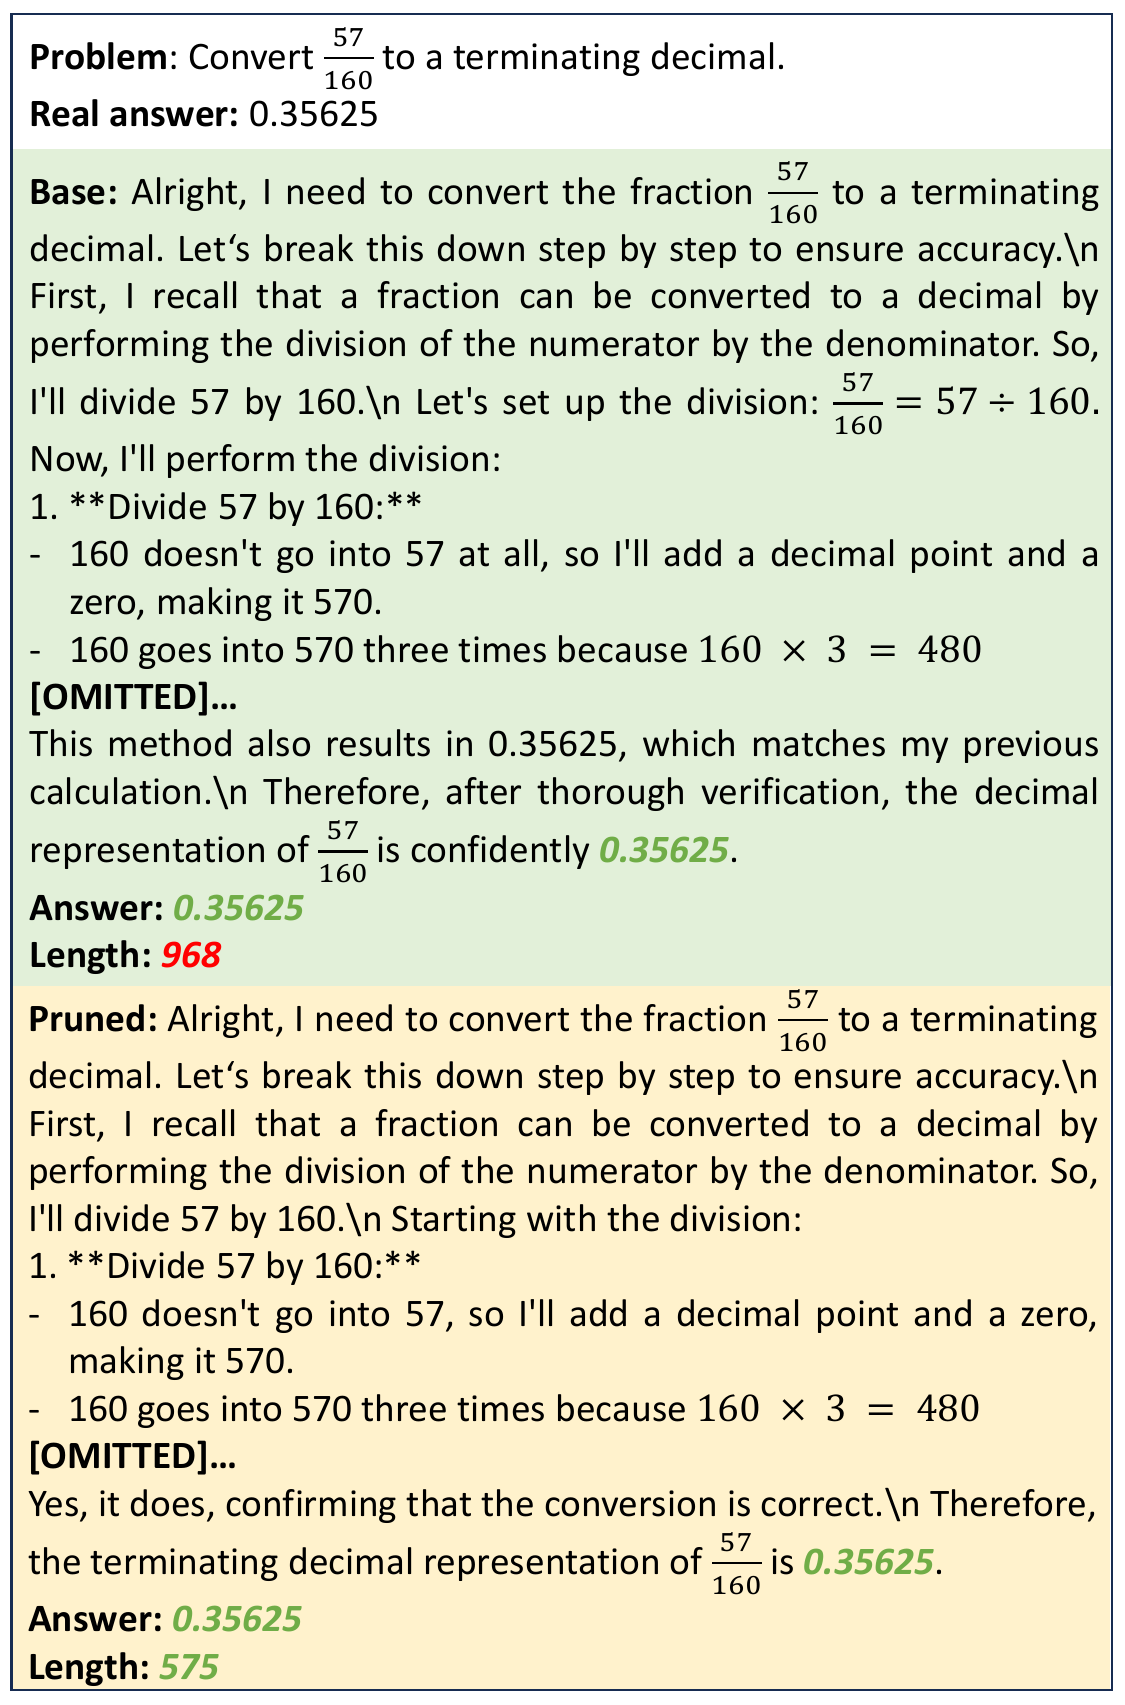}
% \vspace{-12mm}
% \caption{Model Architecture.}
\vspace{-0.2cm}
\caption{case 1 (Marco-o1-7B)} 
\label{fig:case1}
\end{figure*}

\begin{figure*}[htbp]
\centering
\includegraphics[width=5.5in]{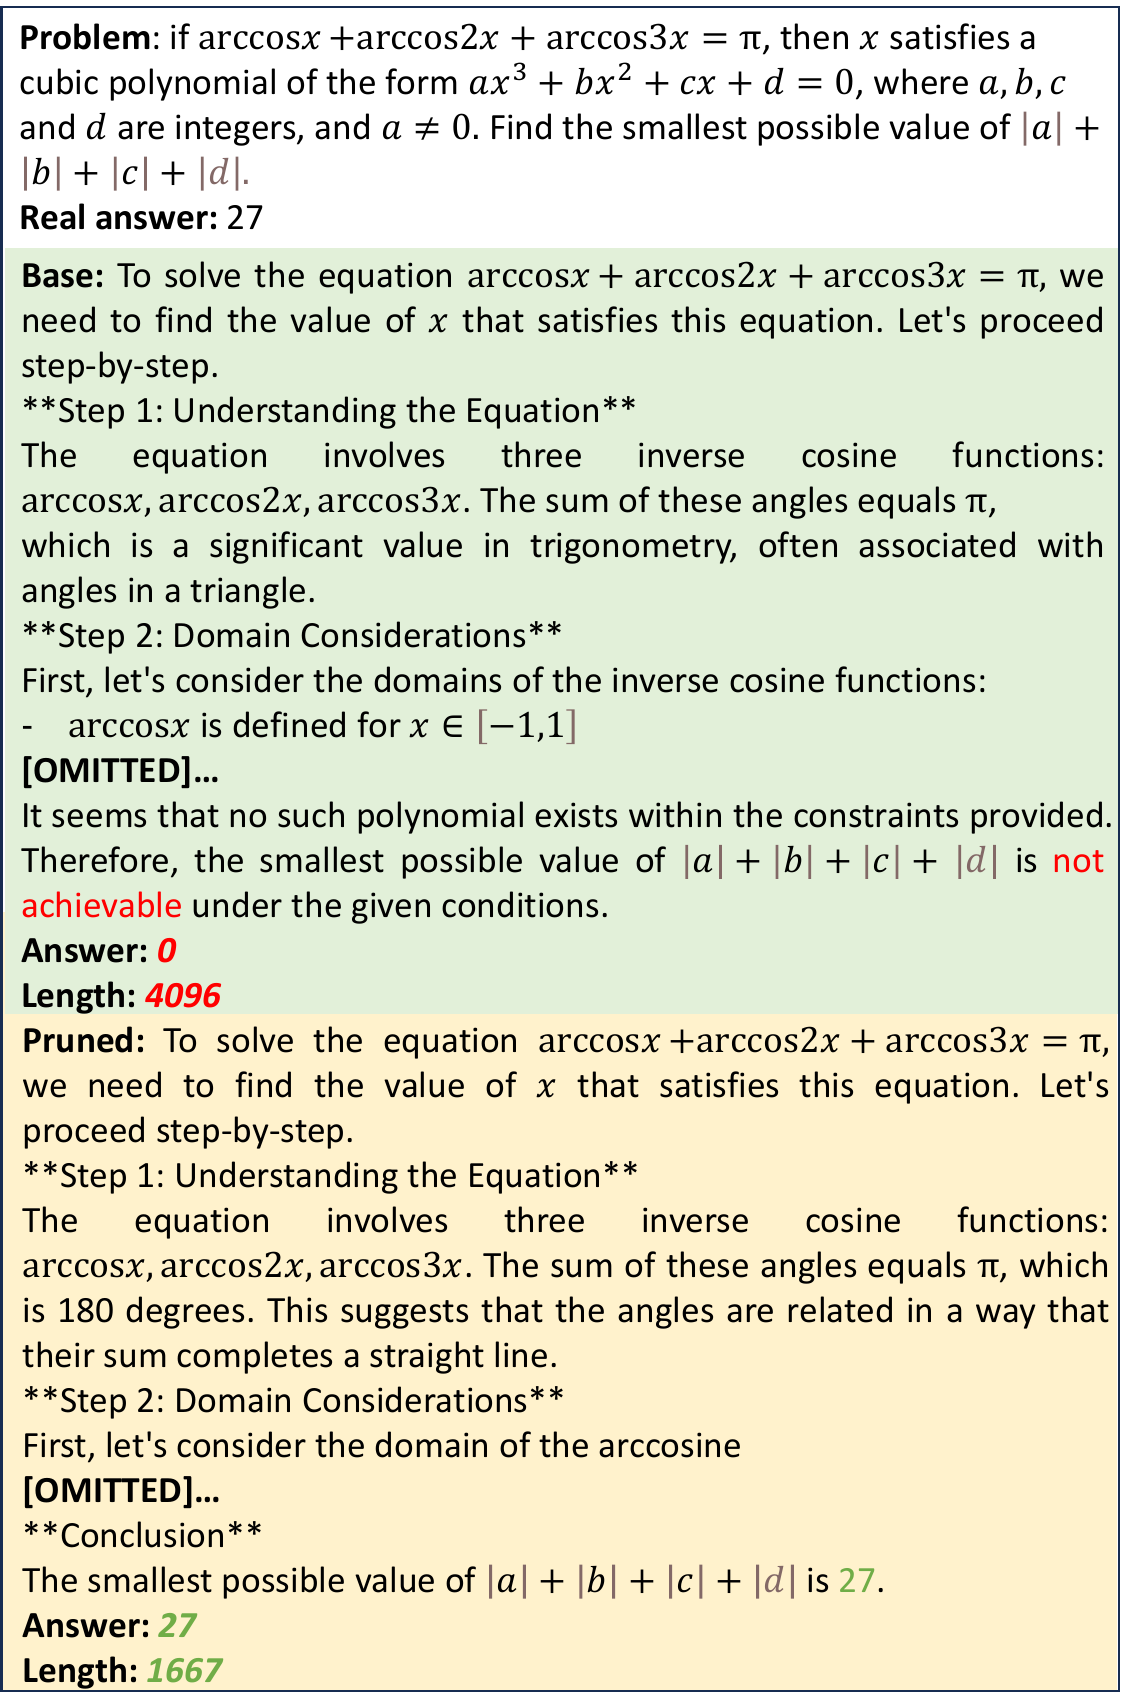}
% \vspace{-12mm}
% \caption{Model Architecture.}
\vspace{-0.2cm}
\caption{case 2 (Marco-o1-7B)} 
\label{fig:case2}
\end{figure*}

\begin{figure*}[htbp]
\centering
\includegraphics[width=5.5in]{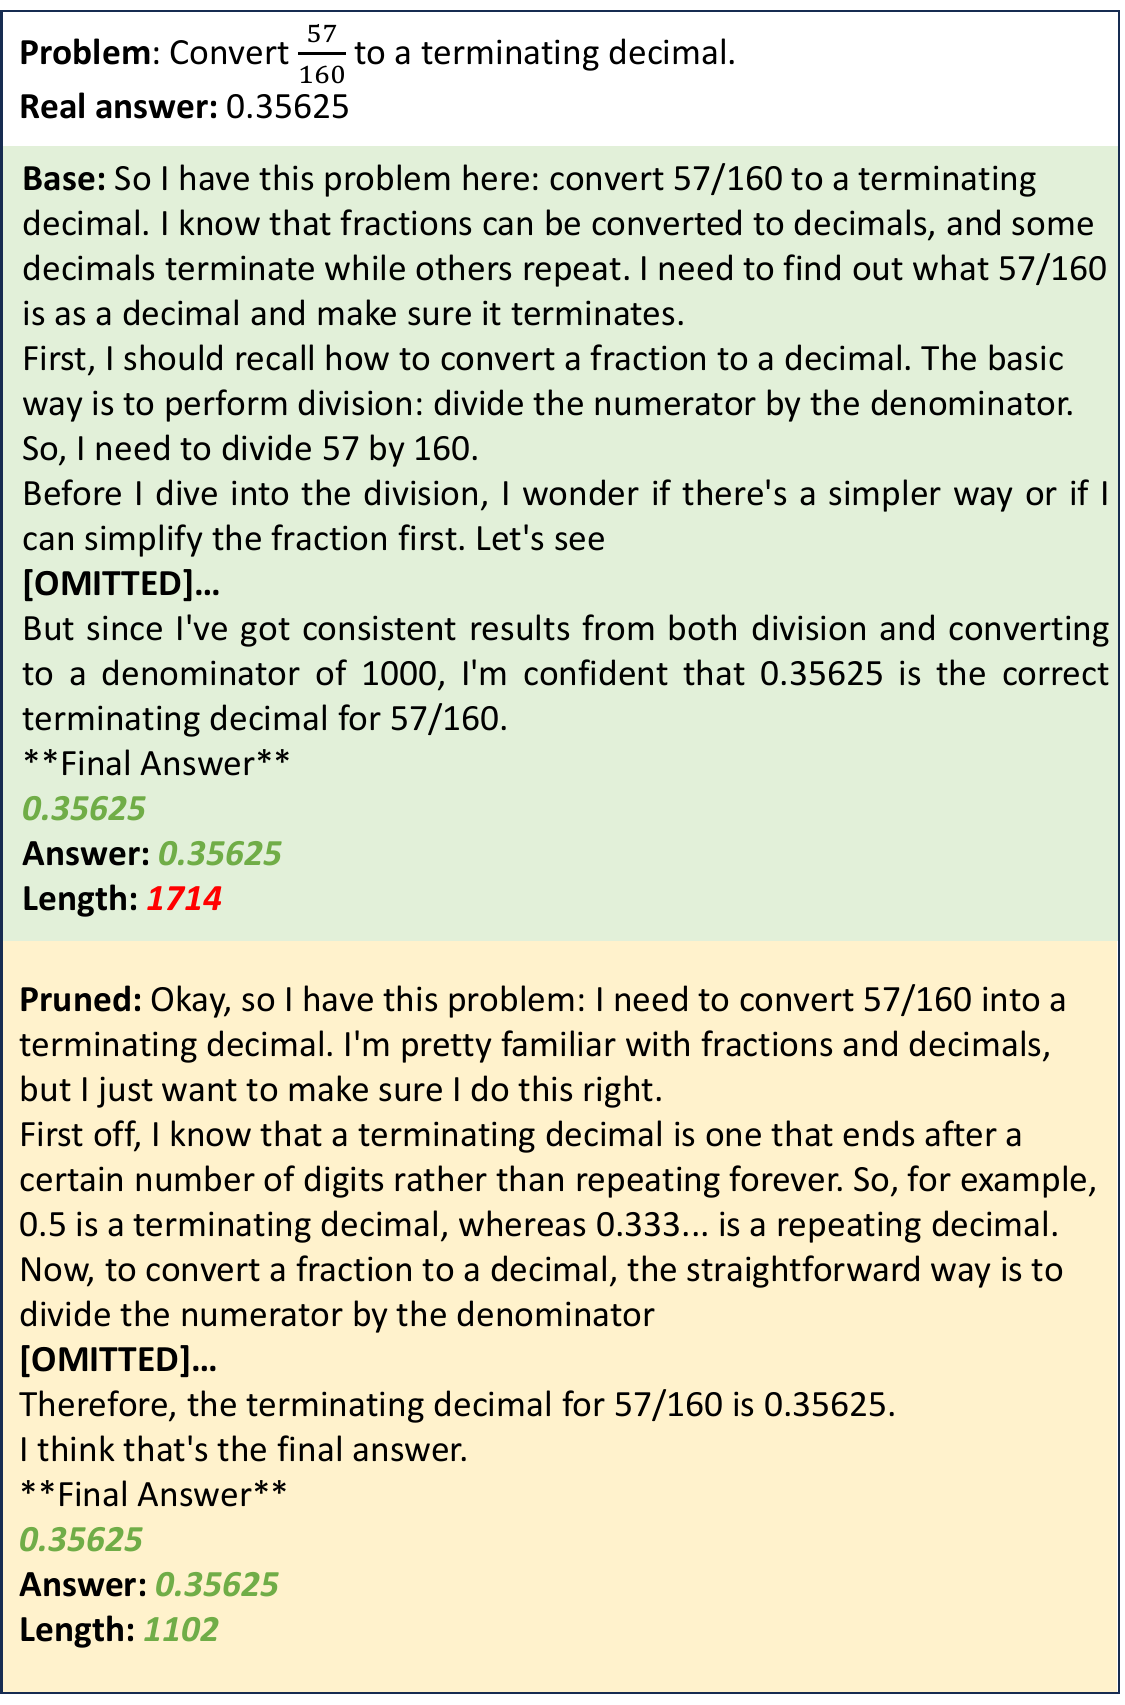}
% \vspace{-12mm}
% \caption{Model Architecture.}
\vspace{-0.2cm}
\caption{case 3 (QwQ-32B-Preview)} 
\label{fig:case3}
\end{figure*}

\begin{figure*}[htbp]
\centering
\includegraphics[width=5.5in]{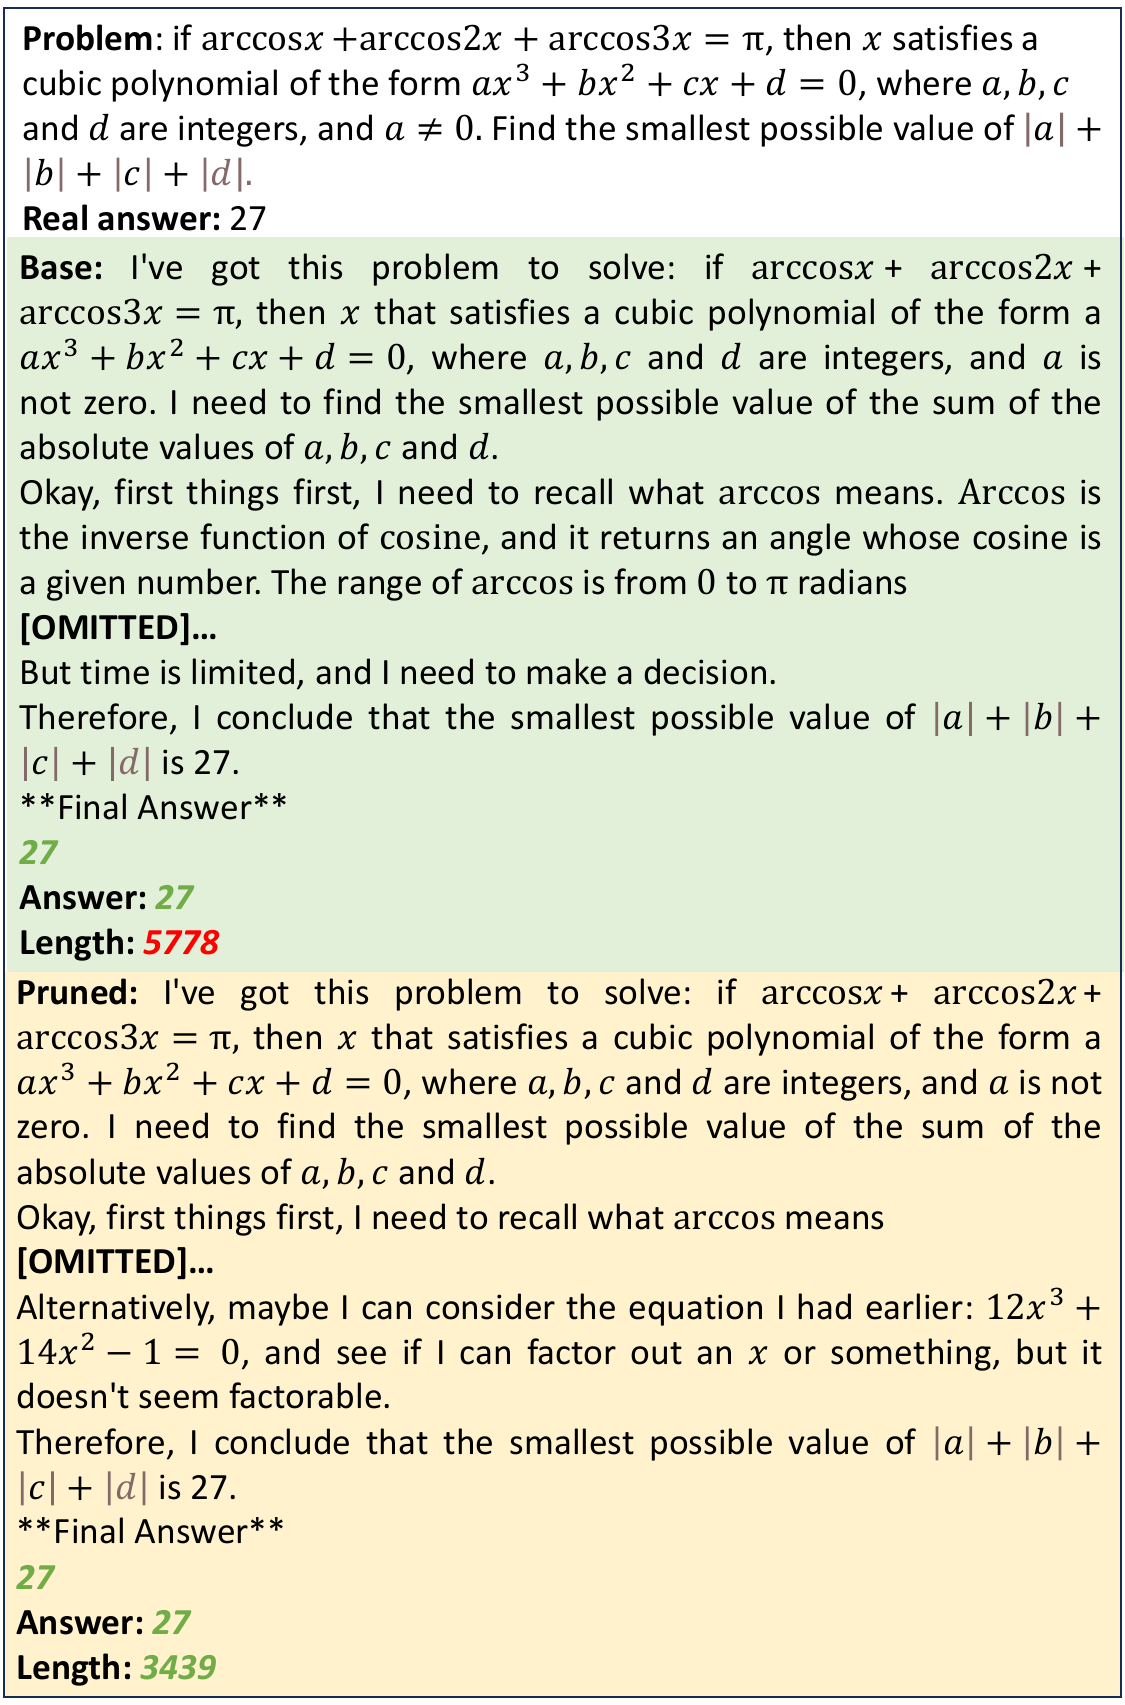}
% \vspace{-12mm}
% \caption{Model Architecture.}
\vspace{-0.2cm}
\caption{case 4 (QwQ-32B-Preview)} 
\label{fig:case4}
\end{figure*}
