# Supplementary material for: O1-Pruner: Length-Harmonizing Fine-Tuning for O1-Like Reasoning Pruning
Source: arXiv:2501.12570 source file (2025-01-29)
Supplement: Supplementary file 2 [file appendix.tex]

\newpage
\appendix
\onecolumn
\section{Appendix}

\subsection{Training Details}

\subsection{Generated Samples}
